# Supplementary material for: Understanding how people consume low quality and extreme news using web traffic data
Source: arXiv:2201.04226 source file (2022-01-11)
Supplement: Supplementary file 1 [file appendix.tex]

% \clearpage
% \section{Appendices}
\appendix
\section{Appendices}
\label{section:appendix}
\subsection{Significance tests for the mean number of visitors to~\gp from Swing, Republican and Democratic states.}

In Finding 3, we mention that people from Swing and Republican states are more likely to visit~\gp than people from Democratic states. To validate our hypothesis, we first perform a one-way ANOVA test. The null hypothesis is that all three types of states have the same population mean. When we use absolute visitor count, the p-value is $0.06$; when we use per-capita visitor count, the p-value is $1.5\mathrm{e}{-7}$. We choose p-value = $0.01$ as a threshold to reject any null hypothesis. The ANOVA test tells us that on absolute count level, there is no significant difference on the average number of visitors from Swing, Republican and Democratic states. On a per-capita level, at least one type of state has a different mean from others.

To understand which type of state is different. We then perform pairwise t-tests. For each pairwise comparison, the null hypothesis is that the two type of states (e.g., Swing versus Republican, or Republican versus Democratic) have the same per-capita average number of visitors to~\gp. 

Table~\ref{table:state-level-swing-rep-dem-ttest} shows p-values of all pairwise comparisons. There are significantly more visitors from Swing and Republican states who visit~\gp than from Democratic states. However, the difference between Swing and Republican states is not statistically significant (p-value = $0.77 > 0.01$).

% We use a Python statistical package called \textit{scikit-posthocs}.\footnote{For reference, check \url{https://scikit-posthocs.readthedocs.io/en/latest/}}. We use a p-value of $0.01$.

% [refer to python software and configuration]

\begin{table}[t]
\begin{tabular}{p{0.30\linewidth}|p{0.19\linewidth}p{0.18\linewidth}p{0.18\linewidth}}
\toprule
State's voting preference & Swing & Republican & Democratic \\
\midrule
 Swing &  1	& 0.77 & $1.19\mathrm{e}{-8}$ \\
  Republican  &  0.77	& 1 & $7.44\mathrm{e}{-6}$ \\
  Democratic  &  $1.19\mathrm{e}{-8}$ & $7.44\mathrm{e}{-6}$ & 1  \\
\bottomrule
\end{tabular}
\caption{Pairwise t-tests. The variable of interest is the mean number of visitors (per-capita) from each type of state. There are significantly more visitors from Swing and Republican states than from Democratic states.}
\label{table:state-level-swing-rep-dem-ttest}
\end{table}
